# Supplementary material for: Signatures of Electron Fractionalization in Ultraquantum Bismuth
Source: arXiv:0802.1993 source file (2008-02-14)
Supplement: Supplementary file 1 [file Supportingonlinematerial.pdf]

# Supporting online material for "Signatures of electron fractionalization in ultraquantum bismuth"

Kamran Behnia[1], Luis Balicas[2] and Yakov Kopelevich[3]

[1] Laboratoire de Photons et matière (CNRS-UPR5), ESPCI, 10, Rue Vauquelin, 75231 Paris, France

[2] National High Magnetic Field Laboratory, Florida State University, Tallahassee, Florida 32306, USA

[3] Instituto de Fisica ``Gleb Wataghin'', UNICAMP, 13083-970 Campinas, São Paulo, Brazil

## Method of measurement

The Nernst effect was measured with a miniature two-thermometer-one-heater setup designed to function in the reduced space of a 33 T resistive magnet. One end of the sample was anchored to the cold finger and a heat current was applied along the sample with a heater. Thermal gradient across the sample (as well as the average temperature of the sample in presence of the heat current) were measured with two $RuO_2$ thermometers. In our range of study, the thermal conductivity of bismuth is dominated by phonons whose contribution exceeds the electronic one by several orders of magnitude [S1]. This leads to a considerable simplification. As the thermal conductivity of the sample is field-independent in our range of study, there is no need for a precise calibration of the thermometers in strong magnetic fields. Instead, the temperature gradient along the sample was measured at zero field for a given magnitude of applied heat current and the latter was then kept constant during each field sweep. Monitoring the resistance of the two thermometers during each field sweep, we checked that the temperature gradient did not show any detectable (~ 1 percent) oscillations. For all temperatures, the temperature difference along the sample was kept less than 2 percent of its average temperature (at T= 0.56K, $\Delta$T~ 2 mK).

## Sample characterization

The sample used in this study was the same used in our previous low-field studies [S1, S2]. Its dimensions were 4 X 2.1 X 0.8 mm$^3$. The ratio of room temperature to residual resistivity (RRR) was 47 and its residual resistivity was $\rho_0$= 2.5 $\mu\Omega$ cm. The [elastic] mean-free-path is estimated to be about 40 µm. Note that the inelastic mean-free-path is an order of magnitude longer and approaches the sample dimensions. The temperature dependence of the resistivity and thermal conductivity of our sample can be found in ref. S1. We also measured the magnetoresistance of our sample up to 33T (See Fig. S1). The field-induced increase in resistivity is $\Delta\rho$ (B=33 T) / $\rho$ (B=0)

= 3.3 $10^5$. This is close to with what was found in a previous study [S3] for this field orientation at T=4.2K.

# Electronic mobility

Assuming an equal mobility of electrons and holes and a carrier density of 3 $10^{17}$ $cm^3$ for each type of carriers, a residual resistivity of 2.5 $\mu\Omega$ cm would imply a mobility of $\mu_h$=$\mu_e$= 4.2 $10^6$ $cm^2s^{-1}V^{-1}$. However, the hole mobility exceeds by far the electron mobility and this implies a $\mu_h$ as large as 8 $10^6$ $cm^2s^{-1}V^{-1}$. It is instructive to recall that the GaAs/AlGaAs sample in which the FQHE was discovered had a mobility of 9 $10^4$ $cm^2s^{-1}V^{-1}$ [S4] , almost two orders of magnitude lower. On the other hand, Bi crystals studied decades ago had RRRs as large as 595 [S5] indicative of a mobility exceeding ours by an order of magnitude.

# Quantum limit in Bi for a field along the trigonal axis

Before firmly concluding that the quantum limit is attained in bismuth by applying a field of 9T along the trigonal axis, one should consider several issues:

### *a) The field-induced change in the cyclotron frequency:*

When a Landau level of the electronic pockets pulls the chemical potential, the hole Fermi surface responds by a modification in its size in order to keep charge neutrality [S6]. This feature leads to a detectable change in the periodicity of quantum oscillations with increasing magnetic field. The extremal cross sections of the hole and electron ellipsoids (see S7), are calculated using the dHvA frequency at low fields (B < 2 T), namely 0.117 $T^{-1}$ for electrons and 0.157$T^{-1}$ for holes [S8, S9] (see also S9 and S10). According to the studies extended to the quantum limit [S2, S11], the period of oscillations for holes becomes 0.147$T^{-1}$ at high fields. This would slightly enhance the quantum limit.

### *b) The Zeeman splitting:*

It is unusually large in our context of investigation [S6, S10]. The large ratio of Zeeman energy to the cyclotron energy ($\varepsilon_Z$=2.16$\hbar\omega_c$) leads to a drastic change in the $B^{-1}$ position of the anomalies associated with the hole Fermi surface. The anomaly associated with the $0^+$ level is thus pushed to a field *lower* than the $2^-$ one. This feature, first reported in S11, has been also detected in the Nernst measurements [S2]. All available reports converge to find that the $1^-$ anomaly occurs at a field close to 9T (See table S1). Note also that the large Zeeman splitting pushes the $0^-$ anomaly to an infinite field. Therefore, no other integer peak is expected beyond 9T and this sets the quantum limit for holes.

### *c) Absence of oscillations corresponding to the electron ellipsoids:*

Finally, one should consider the invisibility of the frequency associated with the electron ellipsoids in this configuration. For all other field directions, the SdH

frequency of the electronic ellipsoids can be detected even if they are less mobile compared to holes as reflected in their larger Dingle temperature. Moreover, the angular dependence of this frequency is in very good agreement with the shape of the cigar-like ellipsoids [S6, S9]. Intriguingly, however, this frequency disappears when the field aligns the trigonal axis [S6, S8, S9]. One possibility is a resonance between electron and hole frequencies for this configuration. The two frequencies are close to each other. The $B^{-1}$ position of the $1^-$ hole peak (0.112 $T^{-1}$) is almost identical to the expected period associated with the electron orbit (0.117 $T^{-1}$).

Therefore, it is safe to assume that the quantum limit for both electrons and holes is attained at a field close to 9 T. Table S1 resumes the field position of the $1^-$ anomaly which sets the quantum limit detected by various groups. From this data, we conclude that $B_{QL}$ = 8.85 ±0.25 T.

| Probe | T(K) | $B_{QL}$ (T) | Ref. |
|---|---|---|---|
| Resistivity | 1.4 | 8.9 | S6 |
| resistivity | 4.2 | 8.6 | S3 |
| resistivity | 0.06 | 8.62 | S12 |
| resistivity | 0.025 | 9.09 | S11 |
| Nernst | 0.28 | 9 | S2 |

Table S1: Quantum limit for a field along trigonal according according to different studies. $B_{QL}$ is defined as the field at which the first Zeeman-split Landau level ($1^-$) was observed.

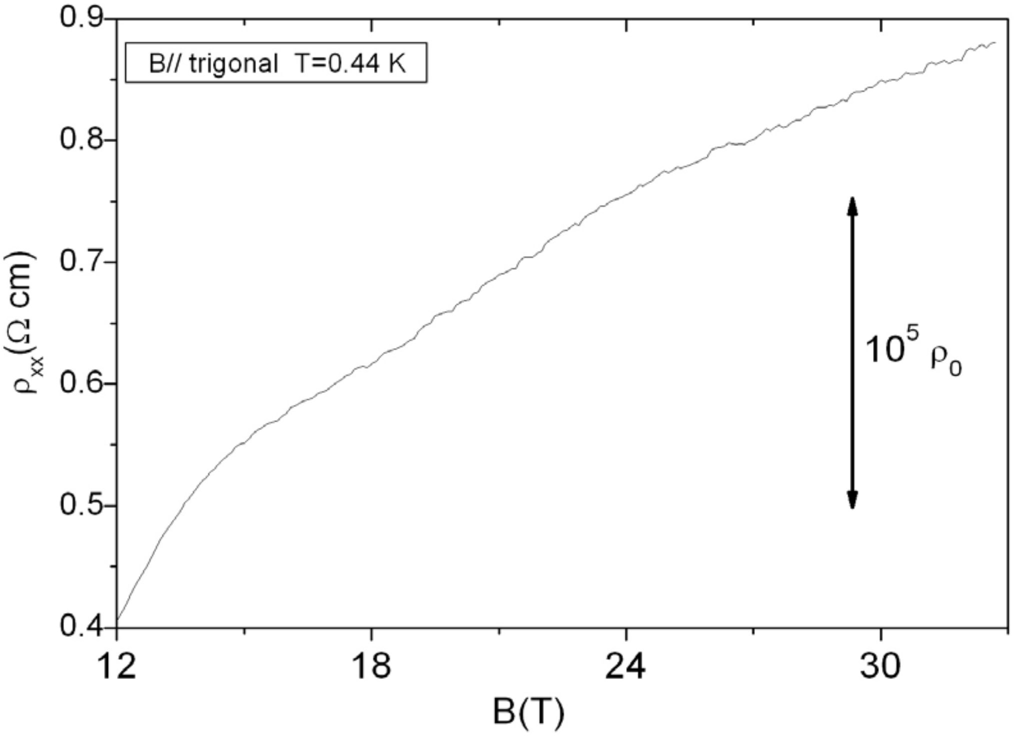


Fig. S1 The high-field magnetoresistance of the sample at 0.44 K. Besides a fuzzy structure, no feature can be definitely resolved beyond the quantum limit.

## Previous evidence for quantized Hall effect in bulk crystals

In contrast to the fractional quantum Hall effect, the integer quantum Hall effect has been previously reported in a number of bulk systems. The case for Quantum Hall Effect in three dimensions was first established by its experimental observation in a GaAs/AlGaAs supperlattice system [S13]. A number of bulk systems are known to display quantized Hall effect [S14-S18]. Bechgaard salts are a celebrated example. In their Field-Induced-Spin-Density-Wave state, they show plateaus of $\rho_{xy}$ [S14, S15]. Similar features have also been reported in the quasi-two-dimensional $\eta$–$Mo_4O_{11}$ [S16] as well as in the layered semiconductor $(Bi_{0.25}Sb_{0.75})_2Te_3$ [S17, S18].

All these studies were performed well below the quantum limit, on strongly anisotropic systems and with electronic mobilities much lower than pure elemental bismuth.

## References


**S1.** K. Behnia, M. -A. Méasson, Y. Kopelevich, Phys. Rev. Lett. **98**, 076603 (2007).

**S2.** K. Behnia, M. -A. Méasson, Y. Kopelevich, Phys. Rev. Lett. **98**, 166602 (2007).

**S3.** K. Hiruma, G. Kido, N. Miura, Solid State Commun. **31**, 1019 (1979)

**S4.** H. L. Stormer, Rev. Mod. Phys. **71**, 875 (1999).

**S5.** J. Boxus C. Uher, J. Heremans, J -P. Issi, Phys. Rev. B **23**, 449 (1981).

**S6.** G. E. Smith, G. A. Baraff and J. M. Rowell, Phys. Rev. **135**, A1118 (1964).

**S7.** D. Shoenberg, Magnetic Oscillations in Metals, Cambridge University Press, Cambridge, 1984, page 233.

**S8.** R. N. Bhargava, Phys. Rev. **156**, 785 (1967).

**S9.** R. D. Brown III, Phys. Rev. B **2**, 928 (1970).

**S10.** V. S. Edelman, Adv. Phys. **25**, 555 (1976).

**S11.** S. G. Bompadre, C. Biagini, D. Maslov, A. F. Hebard, Phys. Rev. B **64**, 073103 (2001).

**S12.** F. Y. Yang *et al.* , Phys. Rev. B **61**, 6631 (2000).

**S13.** H. L. Stormer, J. P. Eisenstein, A. C. Gossard, W. Wiegmann, K. Baldwin, Phys. Rev. Lett. **56**, 85 (1986).

**S14.** J. R. Cooper, W. Kang, P. Auban, G. Montambaux, D. Jérome, K. Bechgaard, Phys. Rev. Lett. **63**, 1984 (1989).

**S15.** S. T. Hannahs, J. S. Brooks, W. Kang, L. Y. Chiang, P. M. Chaikin, Phys. Rev. Lett. **63**,1988 (1989).

**S16.** S. Hill *et al.*, Phys. Rev. B **58**, 10778 (1998).

**S17.** D. Elefant, G. Reiss, Ch. Baier, Eur. Phys. J. B **4** , 45 (1998).

**S18.** N. Miyajima *et al.*, J. Low Temp. Phys. **123**, 219 (2001)
